# Supplementary material for: Think Big, Generate Quick: LLM-to-SLM for Fast Autoregressive Decoding
Source: arXiv:2402.16844 source file (2024-07-17)
Supplement: Supplementary file 1 [file appendices.tex]

\clearpage
\setcounter{section}{0}
\section*{Appendix}

\section{PEFT hyperparameters}
\label{sec:peft_hyperparam}
\hyperref[table:peft_hyperparam]{Table~\ref{table:peft_hyperparam}} presents the hyperparameters for the prompt tuning, prefix tuning, and LoRA methods we considered in the parameter-efficient fine-tuning ablation in our paper.

\begin{table}[hbt!]
\centering
\noindent\adjustbox{max width=\linewidth}{
\begin{tabular}{lll}
\toprule
\belowrulesepcolor{my-gray}
\rowcolor{my-gray}
& \textbf{GPT2} & \textbf{T5 Small}\\
\aboverulesepcolor{my-gray}
\midrule
\textbf{Prompt tuning} & &  \\
\# prompt tokens & 200 & 1024\\
\midrule
%\belowrulesepcolor{my-gray}
%\rowcolor{my-gray}
%& \textbf{GPT2} & \textbf{T5 Small}\\
\textbf{Prefix tuning} & & \\
\# prefix tokens & 256 & 1024\\
project. hidden size & 64 & 64\\
\midrule
%\belowrulesepcolor{my-gray}
%\rowcolor{my-gray}
\textbf{LoRA} & & \\
Rank & 40 & 24\\
$\alpha$ & 64 & 32\\
Dropout & 0.1 & 0.1\\
\bottomrule
\end{tabular}
}
\caption{Hyperparameters for prompt tuning, prefix tuning and LoRA.}
\label{table:peft_hyperparam}
\end{table}

\section{Using decoder-only models as LLM}
\label{sec:appendix_decoder_only}
We present preliminary result for using decode-only models as an LLM in our \methodname{} framework on the summarization task. We use GPT2 XL as the LLM and GPT2 base as the SLM in our experiments. Compared to Encoder-Decoder based LLMs, there is no specific layer in the model which can explicitly be identified as the encoded representation of the prompt. Therefore, we experiment with extracting representations from different layers of the GPT XL model before passing it to the projector and subsequently to the SLM. The results are presented in \hyperref[tab:summarization_decoder]{Table~\ref{tab:summarization_decoder}}. Surprisingly, we observe that

\begin{table}[hbt!]
\centering
\noindent\adjustbox{max width=\linewidth}{
\begin{tabular}{llllll}
\toprule
\textbf{Model} & \textbf{R-1} & \textbf{R-2} & \textbf{R-L} & \textbf{Avg.}\\
\midrule
GPT2-XL & 40.47 & 19.09 & 28.90 & 29.49 \\ %37.94  \\
GPT2 & 38.58 & 17.56 & 27.36 & 27.83 \\ %36.06 \\
\midrule
GPT2-XL-2-GPT2 (layer 0) & 39.16 & 17.71 & 27.43 & 36.55 \\ %37.64\\
GPT2-XL-2-GPT2 (layer 1) & 39.05 & 17.63 & 27.40 & 36.43 \\ %37.64\\
GPT2-XL-2-GPT2 (layer 4) & 36.66 & 16.46 & 25.64 & 34.87 \\ %37.64\\
GPT2-XL-2-GPT2 (layer 8) & 33.27 & 14.03 & 23.24 & 30.98 \\ %37.64\\
GPT2-XL-2-GPT2 (all layers, weighted avg) & 37.69 & 16.72 & 26.41 & 35.15 \\ %37.64\\\textbf{}
\aboverulesepcolor{my-blue}
%\textcolor{red}{GPT2-XL-2-GPT2} & . & . & . & .\\
\bottomrule
\end{tabular}
}
\caption{ROUGE scores (abbreviated with R-) on CNN/Daily Mail. GPT2-XL (zero-shot) results are from~\citet{radford2019language}. Runtimes are reported in seconds for 100 generated tokens. \color{red}{TODO: Add proper averaging instead of R-AVG}}
\label{tab:summarization_decoder}
\end{table}

\section{MT-Bench qualitative evaluation}
In this section, we present sample qualitative responses by the baseline LLM, SLM, and our proposed \methodname{} on MT-Bench and their corresponding ratings provided by GPT-4 as the judge.
\label{sec:appendix_mtbench}

\input{tables/MTBenchQualitative}
